# Supplementary material for: Molecular Dipole Moment Learning via Rotationally Equivariant Gaussian Process Regression with Derivatives in Molecular-orbital-based Machine Learning
Source: arXiv:2205.15510 source file (2022-05-31)
Supplement: Supplementary file 1 [file SI_MOB-ML_dipole.pdf]

# Supporting Information for Molecular-orbital-based Machine Learning for Molecular Dipole Moment via Gaussian Process Regression with Derivatives

Jiace Sun,[1] Lixue Cheng,[1] and Thomas F. Miller III[2]
[1)]Division of Chemistry and Chemical Engineering, California Institute of Technology, Pasadena, CA 91125, USA
[2)]Division of Chemistry and Chemical Engineering, California Institute of Technology, Pasadena, CA 91125, USA, tfm@caltech.edu

(Dated: 31 May 2022)

## I. ROTATIONAL EQUIVARIANCE OF DIPOLE MODEL IN THE SINGLE-TASK GPR WITH DERIVATIVES

In this section, we will prove the general single-task GPR with derivatives satisfies rotational equivariance.

For an n-dimensional external variable $\boldsymbol{\alpha} \in \mathbb{R}^n$, we train single-task GPR with derivatives using features $\mathbf{X}_c = (\mathbf{X}, \nabla_{\boldsymbol{\alpha}}\mathbf{X})$ and labels $\nabla_{\boldsymbol{\alpha}}\mathbf{y}$ and generate the predicted distribution $\nabla_{\boldsymbol{\alpha}} f(\mathbf{X}_c^\star)$ on test features $\mathbf{X}_c^\star$. Assume that the transformation of features and labels under rotation operator $\hat{U}$ is given by

$$\hat{U}\mathbf{X} = \mathbf{X}, \hat{U}\nabla_{\boldsymbol{\alpha}}\mathbf{X} = U\nabla_{\boldsymbol{\alpha}}\mathbf{X}, \hat{U}\mathbf{y} = \mathbf{y}, \hat{U}\nabla_{\boldsymbol{\alpha}}\mathbf{y} = U\nabla_{\boldsymbol{\alpha}}\mathbf{y}, \tag{1}$$

we show that $\nabla_{\boldsymbol{\alpha}} f(\mathbf{X}_c^\star)$ satisfies rotational equivariance:

$$\nabla_{\boldsymbol{\alpha}} f(\hat{U}\mathbf{X}_c^\star) = U\nabla_{\boldsymbol{\alpha}} f(\mathbf{X}_c^\star). \tag{2}$$

Proof:

In single-task GPR with derivatives, the kernel matrix element of $x_c = (x, \nabla_{\boldsymbol{\alpha}} x)$, $x'_c = (x', \nabla_{\boldsymbol{\alpha}} x')$ is

$$K_s(x_c, x'_c) = \nabla_{\boldsymbol{\alpha}} x \nabla_x \nabla_{x'} K(x, x')(\nabla_{\boldsymbol{\alpha}} x')^T. \tag{3}$$

Let the Gaussian likelihood covariance to be $\Sigma_s$. The prediction on $\mathbf{X}_c^\star$ is a Gaussian distributed function $\nabla_{\boldsymbol{\alpha}} f(\mathbf{X}_c^\star)$ with the mean and variance

$$\mathbb{E}[\nabla_{\boldsymbol{\alpha}} f(\mathbf{X}_c^\star)] = K_s(\mathbf{X}_c^\star, \mathbf{X}_c)(K_s(\mathbf{X}_c, \mathbf{X}_c) + \Sigma_s)^{-1}\nabla_{\boldsymbol{\alpha}}\mathbf{y}, \tag{4}$$

$$\mathrm{Var}[\nabla_{\boldsymbol{\alpha}} f(\mathbf{X}_c^\star)] = K_s(\mathbf{X}_c^\star, \mathbf{X}_c)(K_s(\mathbf{X}_c, \mathbf{X}_c) + \Sigma_s)^{-1} K_s(\mathbf{X}_c, \mathbf{X}_c^\star). \tag{5}$$

So the rotational equivariance is equivalent to

$$\mathbb{E}[\nabla_{\boldsymbol{\alpha}} f(\hat{U}\mathbf{X}_c^\star)] = U\mathbb{E}[\nabla_{\boldsymbol{\alpha}} f(\hat{U}\mathbf{X}_c^\star)],$$
$$\mathrm{Var}[\nabla_{\boldsymbol{\alpha}} f(\hat{U}\mathbf{X}_c^\star)] = U\mathrm{Var}[\nabla_{\boldsymbol{\alpha}} f(\hat{U}\mathbf{X}_c^\star)]U^T.$$

Note that

$$K_s(\hat{U}\mathbf{X}_c^\star, \mathbf{X}_c) = U\nabla_{\boldsymbol{\alpha}}\mathbf{X}^\star \nabla_{x^\star}\nabla_{\mathbf{X}} K(\mathbf{X}^\star, \mathbf{X})(\nabla_{\boldsymbol{\alpha}}\mathbf{X})^T = UK_s(\mathbf{X}_c^\star, \mathbf{X}_c), \tag{6}$$

$$K_s(\mathbf{X}_c, \hat{U}\mathbf{X}_c^\star) = \nabla_{\boldsymbol{\alpha}}\mathbf{X}\nabla_{\mathbf{X}}\nabla_{x^\star} K(\mathbf{X}, \mathbf{X}^\star)(U\nabla_{\boldsymbol{\alpha}}\mathbf{X}^\star)^T = K_s(\mathbf{X}_c, \mathbf{X}_c^\star)U^T. \tag{7}$$

Thus we have

$$\mathbb{E}[\nabla_{\boldsymbol{\alpha}} f(\hat{U}\mathbf{X}_c^\star)] = K_s(\hat{U}\mathbf{X}_c^\star, \mathbf{X}_c)(K_x(\mathbf{X}_c, \mathbf{X}_c) + \Sigma_s)^{-1}\nabla_{\boldsymbol{\alpha}}\mathbf{y} \tag{8}$$

$$= UK_s(\mathbf{X}_c^\star, \mathbf{X}_c)(K_x(\mathbf{X}_c, \mathbf{X}_c) + \Sigma_s)^{-1}\nabla_{\boldsymbol{\alpha}}\mathbf{y} \tag{9}$$

$$= U\mathbb{E}[\nabla_{\boldsymbol{\alpha}} f(\mathbf{X}_c^\star)] \tag{10}$$

and

$$\mathrm{Var}[\nabla_{\boldsymbol{\alpha}} f(\hat{U}\mathbf{X}_c^\star)] = K_s(\hat{U}\mathbf{X}_c^\star, \mathbf{X}_c)(K_x(\mathbf{X}_c, \mathbf{X}_c) + \Sigma_s)^{-1} K_s(\mathbf{X}_c, \hat{U}\mathbf{X}_c^\star) \tag{11}$$

$$= UK_s(\mathbf{X}_c^\star, \mathbf{X}_c)(K_x(\mathbf{X}_c, \mathbf{X}_c) + \Sigma_s)^{-1} K_s(\mathbf{X}_c, \mathbf{X}_c^\star)U^T \tag{12}$$

$$= U\mathrm{Var}[\nabla_{\boldsymbol{\alpha}} f(\hat{U}\mathbf{X}_c^\star)]U^T. \tag{13}$$

which finish the proof.

In MOB-ML dipole learning, the features $\boldsymbol{f}_{ij}^{\boldsymbol{\mu}} = \{\boldsymbol{f}_{ij}^{\varepsilon}, \nabla_{\mathscr{E}}\boldsymbol{f}_{ij}^{\varepsilon}\}$ and the pair dipole moment labels satisfy the condition in Eq. 1, thus the prediction $\boldsymbol{\mu}^{\mathrm{ML}}$ is rotational equivariant.

## II. ROTATIONAL INVARIANCE OF ENERGY MODEL AND ROTATIONAL EQUIVARIANCE OF DIPOLE MODEL IN THE MULTI-TASK GPR WITH DERIVATIVES

In this section, we show the energy and dipole model satisfy rotational invariance and equivariance, respectively, in the multi-task GPR with derivatives.

For an n-dimensional external variable $\boldsymbol{\alpha} \in \mathbb{R}^n$, we train multi-task GPR with derivatives using features $\mathbf{X}_c = (\mathbf{X}, \nabla_{\boldsymbol{\alpha}}\mathbf{X})$ and labels $\mathbf{y}_c = (\mathbf{y}, \nabla_{\boldsymbol{\alpha}}\mathbf{y})$ and generate the predicted distribution $\begin{bmatrix} f(\mathbf{X}_c^\star) \\ \nabla_{\boldsymbol{\alpha}} f(\mathbf{X}_c^\star) \end{bmatrix}$ on test features $\mathbf{X}_c^\star$. Assume that the transformation of features and labels under rotation operator $\hat{U}$ is given by

$$\hat{U}\mathbf{X} = \mathbf{X}, \hat{U}\nabla_{\boldsymbol{\alpha}}\mathbf{X} = U\nabla_{\boldsymbol{\alpha}}\mathbf{X}, \hat{U}\mathbf{y} = \mathbf{y}, \hat{U}\nabla_{\boldsymbol{\alpha}}\mathbf{y} = U\nabla_{\boldsymbol{\alpha}}\mathbf{y}, \tag{14}$$

we show that $f(\mathbf{X}_c^\star)$ satisfies rotaional invariance and $\nabla_{\boldsymbol{\alpha}} f(\mathbf{X}_c^\star)$ satisfies rotational equivariance:

$$\begin{bmatrix} f(\hat{U}\mathbf{X}_c^\star) \\ \nabla_{\boldsymbol{\alpha}} f(\hat{U}\mathbf{X}_c^\star) \end{bmatrix} = \begin{bmatrix} f(\mathbf{X}_c^\star) \\ U\nabla_{\boldsymbol{\alpha}} f(\mathbf{X}_c^\star) \end{bmatrix}. \tag{15}$$

Proof:

In multi-task GPR with derivatives, the kernel matrix element for $x_c = (x, \nabla_{\boldsymbol{\alpha}} x)$, $x'_c = (x', \nabla_{\boldsymbol{\alpha}} x')$ is

$$K_m(x_c, x'_c) = \begin{bmatrix} K(x,x') & \nabla_{x'} K(x,x')(\nabla_{\boldsymbol{\alpha}} x')^T \\ \nabla_{\boldsymbol{\alpha}} x \nabla_x K(x,x') & \nabla_{\boldsymbol{\alpha}} x \nabla_x \nabla_{x'} K(x,x')(\nabla_{\boldsymbol{\alpha}} x')^T \end{bmatrix}. \tag{16}$$

Let the Gaussian likelihood covariance to be $\Sigma_m$. The prediction of $\mathbf{X}_c^\star$ is a Gaussian distributed function $\begin{bmatrix} f(\mathbf{X}_c^\star) \\ \nabla_{\boldsymbol{\alpha}} f(\mathbf{X}_c^\star) \end{bmatrix}$ with the mean and variance

$$\mathbb{E}[\begin{bmatrix} f(\mathbf{X}_c^\star) \\ \nabla_{\boldsymbol{\alpha}} f(\mathbf{X}_c^\star) \end{bmatrix}] = K_m(\mathbf{X}_c^\star, \mathbf{X}_c)(K_m(\mathbf{X}_c, \mathbf{X}_c) + \Sigma_m)^{-1}\mathbf{y}_c, \tag{17}$$

$$\mathrm{Var}[\begin{bmatrix} f(\mathbf{X}_c^\star) \\ \nabla_{\boldsymbol{\alpha}} f(\mathbf{X}_c^\star) \end{bmatrix}] = K_m(\mathbf{X}_c^\star, \mathbf{X}_c)(K_m(\mathbf{X}_c, \mathbf{X}_c) + \Sigma_m)^{-1}K_m(\mathbf{X}_c, \mathbf{X}_c^\star). \tag{18}$$

So the rotational equivariance is equivalent to

$$\mathbb{E}[\begin{bmatrix} f(\hat{U}\mathbf{X}_c^\star) \\ \nabla_{\boldsymbol{\alpha}} f(\hat{U}\mathbf{X}_c^\star) \end{bmatrix}] = \begin{bmatrix} I & 0 \\ 0 & U \end{bmatrix} \mathbb{E}[\begin{bmatrix} f(\mathbf{X}_c^\star) \\ \nabla_{\boldsymbol{\alpha}} f(\mathbf{X}_c^\star) \end{bmatrix}], \tag{19}$$

$$\mathrm{Var}[\begin{bmatrix} f(\hat{U}\mathbf{X}_c^\star) \\ \nabla_{\boldsymbol{\alpha}} f(\hat{U}\mathbf{X}_c^\star) \end{bmatrix}] = \begin{bmatrix} I & 0 \\ 0 & U \end{bmatrix} \mathrm{Var}[\begin{bmatrix} f(\mathbf{X}_c^\star) \\ \nabla_{\boldsymbol{\alpha}} f(\mathbf{X}_c^\star) \end{bmatrix}] \begin{bmatrix} I & 0 \\ 0 & U^T \end{bmatrix}. \tag{20}$$

Note that

$$K_m(\hat{U}\mathbf{X}_c^\star, \mathbf{X}_c) = \begin{bmatrix} K(\mathbf{X}^\star, \mathbf{X}) & \nabla_{\mathbf{X}} K(\mathbf{X}^\star, \mathbf{X})(\nabla_{\boldsymbol{\alpha}}\mathbf{X})^T \\ U\nabla_{\boldsymbol{\alpha}}\mathbf{X}^\star \nabla_{x^\star} K(\mathbf{X}^\star, \mathbf{X}) & U\nabla_{\boldsymbol{\alpha}}\mathbf{X}^\star \nabla_{x^\star} \nabla_{\mathbf{X}} K(\mathbf{X}^\star, \mathbf{X})(\nabla_{\boldsymbol{\alpha}}\mathbf{X})^T \end{bmatrix} = \begin{bmatrix} I & 0 \\ 0 & U \end{bmatrix} K_m(\mathbf{X}_c^\star, \mathbf{X}_c), \tag{21}$$

$$K_m(\mathbf{X}_c, \hat{U}\mathbf{X}_c^\star) = \begin{bmatrix} K(\mathbf{X}, \mathbf{X}^\star) & \nabla_{x^\star} K(\mathbf{X}, \mathbf{X}^\star)(U\nabla_{\boldsymbol{\alpha}}\mathbf{X}^\star)^T \\ \nabla_{\boldsymbol{\alpha}}\mathbf{X} \nabla_{\mathbf{X}} K(\mathbf{X}, \mathbf{X}^\star) & \nabla_{\boldsymbol{\alpha}}\mathbf{X} \nabla_{\mathbf{X}} \nabla_{x^\star} K(\mathbf{X}, \mathbf{X}^\star)(U\nabla_{\boldsymbol{\alpha}}\mathbf{X}^\star)^T \end{bmatrix} = K_m(\mathbf{X}_c, \mathbf{X}_c^\star) \begin{bmatrix} I & 0 \\ 0 & U^T \end{bmatrix}. \tag{22}$$

Thus we have

$$\mathbb{E}[\begin{bmatrix} f(\hat{U}\mathbf{X}_c^\star) \\ \nabla_{\boldsymbol{\alpha}} f(\hat{U}\mathbf{X}_c^\star) \end{bmatrix}] = K_m(\hat{U}\mathbf{X}_c^\star, \mathbf{X}_c)(K_m(\mathbf{X}_c, \mathbf{X}_c) + \Sigma_m)^{-1}\mathbf{y}_c, \tag{23}$$

$$= \begin{bmatrix} I & 0 \\ 0 & U \end{bmatrix} K_m(\mathbf{X}_c^\star, \mathbf{X}_c)(K_m(\mathbf{X}_c, \mathbf{X}_c) + \Sigma_m)^{-1}\mathbf{y}_c, \tag{24}$$

$$= \begin{bmatrix} I & 0 \\ 0 & U \end{bmatrix} \mathbb{E}[\begin{bmatrix} f(\hat{U}\mathbf{X}_c^\star) \\ \nabla_{\boldsymbol{\alpha}} f(\hat{U}\mathbf{X}_c^\star) \end{bmatrix}]. \tag{25}$$

and

$$\mathrm{Var}[\begin{bmatrix} f(\hat{U}\mathbf{X}_c^\star) \\ \nabla_{\boldsymbol{\alpha}} f(\hat{U}\mathbf{X}_c^\star) \end{bmatrix}] = K_m(\hat{U}\mathbf{X}_c^\star, \mathbf{X}_c)(K_m(\mathbf{X}_c, \mathbf{X}_c) + \Sigma_m)^{-1} K_m(\mathbf{X}_c, \hat{U}\mathbf{X}_c^\star), \tag{26}$$

$$= \begin{bmatrix} I & 0 \\ 0 & U \end{bmatrix} K_s(\mathbf{X}_c^\star, \mathbf{X}_c)(K_m(\mathbf{X}_c, \mathbf{X}_c) + \Sigma_m)^{-1} K_m(\mathbf{X}_c, \mathbf{X}_c^\star) \begin{bmatrix} I & 0 \\ 0 & U^T \end{bmatrix}, \tag{27}$$

$$= \begin{bmatrix} I & 0 \\ 0 & U \end{bmatrix} \mathrm{Var}[\begin{bmatrix} f(\hat{U}\mathbf{X}_c^\star) \\ \nabla_{\boldsymbol{\alpha}} f(\hat{U}\mathbf{X}_c^\star) \end{bmatrix}] \begin{bmatrix} I & 0 \\ 0 & U^T \end{bmatrix}. \tag{28}$$

which finish the proof.

In MOB-ML energy+dipole learning, the features $\boldsymbol{f}_{ij}^{\boldsymbol{\mu}} = \{\boldsymbol{f}_{ij}^{\varepsilon}, \nabla_{\mathscr{E}} \boldsymbol{f}_{ij}^{\varepsilon}\}$ and the labels (pair energies and pair dipoles) satisfy the condition in Eq. 14, thus the energy prediction $\varepsilon^{\mathrm{ML}}$ is rotational invariant and the dipole prediction $\boldsymbol{\mu}^{\mathrm{ML}}$ is rotational equivariant.

## III. GPR AND GMM/GPR TRAINING PARAMETERS

We note that different parameters are used in AltBBMM and GMM/AltBBMM. In both AltBBMM and GMM/AltBBMM, the block size $s$ in the block conjugate gradient (BCG) is fixed as 50. The BCG iteration stops when all the $s$ relative residuals are smaller than $10^{-6}$. In AltBBMM without GMM, the preconditioner rank is 2500 for energy learning and 5000 for dipole learning. The hyperparameters are optimized from a full GP trained on random 20000 and 5000 pairs for energy and dipole learning, respectively. The noise regularization is set to be $10^{-6}$ and $10^{-4}$ times of the GPR variance for energy and dipole learning, respectively. In GMM/AltBBMM, for both energy and dipole learning, the preconditioner rank in local clusters is 3000 for training of 50000 and 110000 molecules, and is 1500 otherwise. The hyperparameters in local clusters are optimized from a full GP trained on random 20000 and 5000 pairs for energy and dipole learning, respectively. The noise regularization in local clusters is set to be $10^{-10}$ and $10^{-8}$ times of the GPR variance for energy and dipole learning, respectively. However the AltBBMM in some local clusters does not converge or converges slowly. For the AltBBMM calculations that the relative residual does not reach 10% of the first iteration in 100 iterations, the noise regularization is reset to be $10^{-8}$ and $10^{-6}$ times of the GPR variance for energy and dipole learning, respectively.

## IV. ADDITIONAL TABLES

TABLE S1. Prediction accuracies of single-task and multi-task MOB-ML (GPR) models trained and tested on water molecules with a reference theory of MP2/cc-pVTZ. The MAEs of dipole and energies (kcal/mol) are plotted in Fig. 2 in the main text.

| | Dipole only | Energy only | Dipole + Energy | |
|---|---|---|---|---|
| Training sizes | $\lvert\boldsymbol{\mu}\rvert_{\mathrm{MAE}}$ (mDebye) | $E_{\mathrm{MAE}}$ (kcal/mol) | $\lvert\boldsymbol{\mu}\rvert_{\mathrm{MAE}}$ (mDebye) | $E_{\mathrm{MAE}}$ (kcal/mol) |
| 2 | 3.714 | 0.260 | 8.217 | 0.357 |
| 5 | 0.143 | 0.012 | 0.633 | 0.004 |
| 10 | 0.111 | 0.0013 | 0.463 | 0.0011 |
| 30 | 0.010 | 0.00029 | 0.020 | 0.00013 |
| 50 | 0.008 | 0.00016 | 0.016 | 0.00005 |
| 80 | 0.006 | 0.00013 | 0.011 | 0.00003 |
| 100 | 0.002 | 0.00006 | 0.006 | 0.00002 |

TABLE S2. Prediction accuracies of single-task MOB-ML (GPR) and MOB-ML (GMM/GPR) models trained and tested on QM9 dataset with a reference theory of MP2/cc-pVTZ. Both vector and length MAEs (mDebye) of the dipole moments are shown in this table. The length MAEs of dipole and MAEs of energies (kcal/mol) are plotted in Fig. 4A and B in the main text, respectively.

| | MOB-ML (AltBBMM) | | MOB-ML (GMM/AltBBMM) | | | |
|---|---|---|---|---|---|---|
| Training sizes | $\lvert\boldsymbol{\mu}\rvert_{\mathrm{MAE}}$ (mDebye) | $E_{\mathrm{MAE}}$ (kcal/mol) | $\lvert\boldsymbol{\mu}\rvert_{\mathrm{MAE}}$ (mDebye) | $E_{\mathrm{MAE}}$ (kcal/mol) | # of diagonal clusters | # of off-diagonal clusters |
| 100 | 37.61 | 1.160 | 45.58 | 0.989 | 1 | 8 |
| 200 | 37.18 | 0.739 | 40.64 | 0.878 | 1 | 20 |
| 500 | 25.67 | 0.407 | 27.60 | 0.449 | 1 | 50 |
| 1000 | 22.93 | 0.317 | 25.34 | 0.364 | 5 | 85 |
| 2000 | – | 0.255 | 19.15 | 0.249 | 6 | 130 |
| 5000 | – | – | 13.40 | 0.161 | 10 | 220 |
| 10000 | – | – | 10.85 | 0.123 | 14 | 460 |
| 20000 | – | – | 8.07 | 0.093 | 30 | 650 |
| 50000 | – | – | 6.14 | 0.061 | 30 | 650 |
| 110000 | – | – | 4.81 | 0.045 | 30 | 650 |

TABLE S3. Summary of true total and predicted energies and dipole moments. The predicted values are obtained from the best MOB-ML (GMM/GPR) model trained on 110,000 structures

| | | Energy (Hartree) | | Dipole (Debye) | | |
|---|---|---|---|---|---|---|
| Dataset | n | True Total | Predict Total | True length | Predict length | HF length |
| $\alpha$-Helix | 0 | -283.9563 | -283.9569 | 1.051 | 1.045 | 1.187 |
| | 4 | -1114.5472 | -1114.5483 | 14.402 | 14.393 | 16.382 |
| | 7 | – | -1737.5094 | – | 27.573 | 31.584 |
| | 10 | – | -2360.4722 | – | 41.339 | 47.072 |
| | 13 | – | -2983.4383 | – | 53.840 | 61.333 |
| | 16 | – | -3606.4100 | – | 70.950 | 80.211 |
| $\beta$-Strand | 0 | -283.9563 | -283.9569 | 1.051 | 1.045 | 1.187 |
| | 1 | -491.5997 | -491.6005 | 2.859 | 2.872 | 2.655 |
| | 2 | -699.2453 | -699.2463 | 4.863 | 4.877 | 4.409 |
| | 3 | -906.8913 | -906.8928 | 7.232 | 7.258 | 6.467 |
| | 4 | -1114.5376 | -1114.5396 | 9.608 | 9.637 | 8.561 |
| | 5 | -1322.1840 | -1322.1865 | 12.109 | 12.145 | 10.749 |
| | 6 | -1529.8304 | -1529.8334 | 14.617 | 14.662 | 12.962 |
| Polyenoic amino acid | 2 | -399.1988 | -399.2002 | 5.240 | 5.204 | 5.966 |
| | 4 | -553.6586 | -553.6582 | 7.154 | 6.856 | 8.623 |
| | 6 | -708.1216 | -708.1183 | 7.972 | 6.916 | 10.126 |
| | 8 | -862.5844 | -862.5779 | 8.770 | 6.799 | 11.607 |
| | 10 | -1017.0474 | -1017.0380 | 9.289 | 6.193 | 12.779 |
| n-Amino carboxylic acid | 4 | -558.509 2 | -558.5106 | 2.298 | 2.294 | 2.654 |
| | 6 | -715.3965 | -715.3983 | 2.294 | 2.290 | 2.650 |
| | 8 | -872.2838 | -872.2861 | 2.277 | 2.273 | 2.630 |
| | 10 | -1029.1711 | -1029.1739 | 2.310 | 2.305 | 2.670 |
